# Supplementary material for: On Estimating Recommendation Evaluation Metrics under Sampling
Source: arXiv:2103.01474 source file (2021-03-03)
Supplement: Supplementary file 1 [file Appendix.tex]

\section{Minimal Bias Estimator and Bias-Variance Trade-off}

\subsection{Minimal Bias Estimator}
In ~\cite{Walid}, Walid try to optimize the average bias of $\mathcal{M}(R)$, that is:
\begin{equation}
\begin{split}
   \widehat{\mathcal{M}}_r&= \arg\min_{\widehat{\mathcal{M}}\in \mathbb{R}^n}\sum\limits_{R=1}^{N}{P(R)(\E{\big[\widehat{\mathcal{M}}_r|R\big]-\mathcal{M}(R))^2}}\\
   &=\arg\min_{\widehat{\mathcal{M}}\in \mathbb{R}^n}\sum\limits_{R=1}^{N}{P(R)(\sum\limits_{r=1}^{n}{p(r|R)\widehat{\mathcal{M}}_r}-\mathcal{M}(R))^2}
   \end{split}
\end{equation}
where $\widehat{\mathcal{M}} = (\mathcal{M}_1,\dots,\mathcal{M}_r,\dots,\mathcal{M}_n)^T$.

Solution is:
\begin{equation}
     \widehat{\mathcal{M}} = (A^TA)^{-1}A^T\pmb{b}
\end{equation}

where:

\begin{equation}
    \begin{split}
        &A\in \mathbb{R}^{N\times n},\quad A_{R,r} = \sqrt{P(R)}P(r|R)\\
        &\pmb{b}\in \mathbb{R}^N,\quad b_{R} = \sqrt{P(R)}\mathcal{M}(R)
    \end{split}
\end{equation}
\subsection{Bias-Variance Trade-off}
and the bias-variance trade-off is:

\begin{equation}
    \widehat{\mathcal{M}}_r&= \arg\min_{\widehat{\mathcal{M}}\in \mathbb{R}^n}\sum\limits_{R=1}^{N}{P(R)\Big((\E{\big[\widehat{\mathcal{M}}_r|R\big]-\mathcal{M}(R))^2  +\gamma \text{Var}[\widehat{\mathcal{M}}_r|R ] }\Big)}
\end{equation}
solution is :
\begin{equation}
\widehat{\mathcal{M}} = \Big((1.0-\gamma)A^TA+\gamma \text{diag}(\pmb{c})  \Big)^{-1}A^T\pmb{b}
\end{equation}
When $\gamma = 1$, solution is:

\begin{equation}
    \widehat{\mathcal{M}}_r = \sum\limits_{R=1}^{N}{\mathcal{M}(R)P(R|r)}
\end{equation}

\section{Rank Order Estimation}\label{ap:rank}

In the book ~\cite{nonparametric}, 
\subsection{Assumption}
$X_1 , X2 , \dots, X_n$ are a random sample from a distribution $F$ with probability measure $P$, where $P((−\infty, x]) = F(x)$. Let the prior guess of the unknown $P$ be the measure $\mu$, and let $\alpha$ denote the degree of confidence in $\mu$. The parameter $\alpha$ is often referred to as the prior sample size.
\subsection{Rank Order Problem}
We let $X_1,\dots,X_n$ be a sample of size $n$ from $F$. The problem is to estimate the rank order $G$ of $X_1$ among $X_1,\dots,X_n$ from the knowledge of $r$ observed values $X_1,\dots, X_r$ with $r < n$. Without loss of generality we can consider $X_1, \dots , X_r$ to be the first $r$ values in the unordered sample.

\subsection{Bayes Optimality of $\widehat{G}$}
let
\begin{itemize}
\item[] K = number of observations of $X_1,\dots , X_n$ less than $X_1$.\\
\item[] L = number of observations of $X_1,\dots , X_n$ equal to $X_1$.\\
\item[] M = number of observations of $X_1,\dots , X_n$ greater than $X_1$.\\
\end{itemize}
Using average ranks when ties are present, the rank order $G$ of $X_1$ among $X_1,\dots,X_n$ is the average of the ranks that would be assigned to the $L$ values tied at $X_1$, in a joint ranking from least to greatest, that is,
\begin{equation}
    G=\frac{(K +1)+(K +2)+\cdots+(K +L)}{L}=K + \frac{L+1}{2}
\end{equation}
In a similar fashion, we define $K^\prime$ ,$L^\prime$, $M^\prime$ as the number of observations of $X_1,\dots, X_r$ less than, equal to, and greater than $X_1$, respectively, so the rank order of $X_1$ among $X_1,\dots, X_r$ is:
\begin{equation}
G^\prime =K^\prime +\frac{L^\prime +1}{2}.
\end{equation}
For squared-error loss, the mean of the posterior distribution of $G$ , given $X_1 , \dots , X_r$, is the Bayes estimator $\widehat{G}$ of $G$. ~\cite{paper} Campbell and Hollander (1978) showed:
\begin{equation}
    \widehat{G}=\frac{n+\alpha}{r+\alpha}G^\prime-\frac{1}{2}\frac{n-r}{r+\alpha}+(n-r)\big[\alpha\mu(-\infty,X_1)+\frac{1}{2}\mu(\{X_1\})   \big]
\end{equation}
\subsection{Non-Bayesian Competitors of $\widehat{G}$}
Johnson ~\cite{} (1974) introduced non-Bayesian estimators of rank order for the rank order problem. His estimators are 
\begin{equation}
G_F = G^\prime + (n - r)F(X_1)
\end{equation}
for the case when F is known and continuous, and
\begin{equation}
G_u = \frac{n + 1}{r + 1} G^\prime
\end{equation}
for the case when F is unknown.

\section{Beta-Binomial Distribution}\label{ap:bbd}

This section describes the general Beta-Binomial, which is slightly different from our scenario where sample size is $n-1$.

\begin{equation*}
    \mathcal{B}(\alpha, \beta) = \int_0^1{x^{\alpha -1}(1-x)^{\beta-1}dx}, \quad \alpha >0, \beta >0
\end{equation*}
Prior:
\begin{equation*}
   p(\theta|\alpha,\beta) = \frac{1}{
    \mathcal{B}(\alpha, \beta)}\theta^{\alpha -1}(1-\theta)^{\beta -1}, \quad \theta \sim Beta(\alpha, \beta)
\end{equation*}
Likelihood:
\begin{equation*}
     p(x|\theta) = \binom{n}{x}\theta^x(1-\theta)^{n-x}, \quad x|\theta \sim Bin(n, \theta)
\end{equation*}
Joint distribution:
\begin{equation*}
    p(x,\theta) = p(x|\theta)p(\theta)= \frac{\binom{n}{x}}{\mathcal{B}(\alpha, \beta)}\theta^{x+\alpha -1}(1-\theta)^{n+\beta -x -1}
\end{equation*}
Marginal distribution of $x$, also called \textbf{beta-binomial distribution}:
\begin{equation}\label{eq:bb_distribution}
    p(x) = \int_0^1{p(x,\theta)}d\theta= \binom{n}{x}\frac{\mathcal{B}(x+\alpha, n+\beta-x)}{\mathcal{B}(\alpha, \beta)},\quad x\sim BetaBin(n,\alpha,\beta)
\end{equation}

Posterior:
\begin{equation}\label{eq:bb_posterior}
    p(\theta|x) = \frac{p(x,\theta)}{p(x)}=\frac{1}{\mathcal{B}(x+\alpha, n+\beta-x)}\theta^{x+\alpha -1}(1-\theta)^{n+\beta -x -1},\quad \theta|x \sim Beta( \alpha+x, \beta + n -x)
\end{equation}

\section{Moment Method for Beta-Binomial Distribution}\label{ap:moment}
\begin{equation*}
    X\sim BetaBin(n,\alpha,\beta)
\end{equation*}

Given a set of i.i.d. observations $X_1,\dots,X_M$, we are trying to estimate the parameters $\alpha$ and $\beta$. The moments of the Beta-Binomial are:
\begin{equation}\label{eq:bb_mean}
    \mu_1 = \E{[X]} = n\frac{\alpha}{\alpha+\beta}
\end{equation}

\begin{equation}\label{eq:bb_var}
    \text{Var}[X] = \frac{n\alpha\beta}{(\alpha+\beta)^2}\frac{\alpha+\beta+n}{\alpha+\beta+1}
\end{equation}

\begin{equation}\label{eq:bb_mu3}
\begin{split}
    \mu_2 &= \E[X^2]=\text{Var}[X]+(\E{[X]})^2\\
    &=\frac{n\alpha(n\alpha+\alpha+\beta)}{(\alpha+\beta)(\alpha+\beta+1)}
    \end{split}
\end{equation}

We equate $\mu_1$ and $\mu_2$ to the empirical moments:
\begin{equation}\label{eq:m1}
   \widehat{\mu}_1\coloneqq m_1 = \frac{1}{M}\sum\limits_{i=1}^{M}{X_i}
\end{equation}

\begin{equation}\label{eq:mu2}
    \widehat{\mu}_2\coloneqq m_2 = \frac{1}{M}\sum\limits_{i=1}^{M}{X^2_i}
\end{equation}

and solving for $\alpha$ and $\beta$, we get:
\begin{equation}\label{eq:moment_ab}
    \widehat {\alpha } =\frac {nm_{1}-m_{2}}{n({\frac {m_{2}}{m_{1}}}-m_{1}-1)+m_{1}}
\end{equation}

\begin{equation}
    \widehat{\beta } =\frac {(n-m_{1})(n-{\frac {m_{2}}{m_{1}}})}{n({\frac {m_{2}}{m_{1}}}-m_{1}-1)+m_{1}}
\end{equation}

% \section{EM Algorithm for Mixtures of Binomial Model}\label{ap:em}

% Recall \cref{eq:mb_mle}, log likelihood function is:
% \begin{equation}\label{eq:log_mle}
%     \log{\mathcal{L}} = \sum\limits_{u=1}^{M}{\log{\sum\limits_{k=1}^{N}{p(x_u,z_{uk}|\theta_k)}}}
% \end{equation}

% \subsection{E-step}
% \begin{equation}
% \mathcal{Q}(\pmb{\pi},\pmb{\pi}^{old})=\sum\limits_{u=1}^{M}{\sum\limits_{k=1}^{N}{\gamma(z_{uk}) \log{p(x_u,z_{uk}|\theta_k)}}}
% \end{equation}

% where
% \begin{equation*}
%     \gamma(z_{uk})=p(z_{uk}|x_u,\pmb{\pi}^{old})=\frac{{\pi}^{old}_k p(x_u|\theta_k)}{\sum\limits_{j=1}^{N}{\pi^{old}_j p(x_u|\theta_j)}}
%     \quad\text{and}\quad \sum\limits_k^{N}{\gamma(z_{uk})}=1
% \end{equation*}

% \subsection{M-step}
% For the maximization with respect to $\pi_k$, we need to introduce a Lagrange multiplier:
% \begin{equation}
%   \mathcal{Q}^\prime(\pmb{\pi},\pmb{\pi}^{old})=\mathcal{Q}(\pmb{\pi},\pmb{\pi}^{old}) + \lambda (1-\sum\limits_{k=1}^{N}{\pi_k})
% \end{equation}

% \begin{equation}
%     \frac{\partial \mathcal{Q}^\prime(\pmb{\pi},\pmb{\pi}^{old})}{\partial \pi_k}=\sum\limits_{u=1}^{M}{ \frac{\gamma(z_{uk}) }{\pi_k} -\lambda}=0
% \end{equation}
% \begin{equation}\label{eq:lambda_pi}
%     \lambda\pi_k=\sum\limits_{u=1}^M{\gamma(z_{uk})}\triangleq M_k
% \end{equation}
% \begin{equation}\label{eq:lambda}
%     \lambda=\sum\limits_{k=1}^{N}\sum\limits_{u=1}^M{\gamma(z_{uk})}=M
% \end{equation}

% Then from \cref{eq:lambda_pi,eq:lambda}, we obtain:
% \begin{equation}
%     \pi^{new}_k=\frac{M_k}{M}
% \end{equation}

\subsection{EM Algorithm for Weighted Log-Likelihood Function}
Recall \cref{eq:mb_mle}
Weighted log-likelihood function is:
\begin{equation}
    \log{\mathcal{L}} = \sum\limits_{u=1}^{M}{w_u \log{\sum\limits_{k=1}^{N}{p(x_u,z_{uk}|\theta_k)}}}
\end{equation}
where $\sum_{u}^M{w_u}=1$

\subsubsection{E-step}

\begin{equation}
\mathcal{Q}(\pmb{\pi},\pmb{\pi}^{old})=\sum\limits_{u=1}^{M}{w_u \sum\limits_{k=1}^{N}{\gamma(z_{uk}) \log{p(x_u,z_{uk}|\theta_k)}}}
\end{equation}

where
\begin{equation*}
    \gamma(z_{uk})=p(z_{uk}|x_u,\pmb{\pi}^{old})=\frac{{\pi}^{old}_k p(x_u|\theta_k)}{\sum\limits_{j=1}^{N}{\pi^{old}_j p(x_u|\theta_j)}}
\end{equation*}

\subsubsection{M-step}

\begin{equation}
   \mathcal{Q}^\prime(\pmb{\pi},\pmb{\pi}^{old})=\mathcal{Q}(\pmb{\pi},\pmb{\pi}^{old}) + \lambda (1-\sum\limits_{k=1}^{N}{\pi_k})
\end{equation}

\begin{equation}
    \frac{\partial \mathcal{Q}^\prime(\pmb{\pi},\pmb{\pi}^{old})}{\partial \pi_k}=\sum\limits_{u=1}^{M}{ \frac{w_u\gamma(z_{uk}) }{\pi_k} -\lambda}=0
\end{equation}

\begin{equation}
    \lambda\pi_k=\sum\limits_{u=1}^M{w_u\gamma(z_{uk})}\triangleq M_k
\end{equation}
\begin{equation}
    \lambda=\sum\limits_{k=1}^{N}\sum\limits_{u=1}^M{w_u\gamma(z_{uk})}=1
\end{equation}

\begin{equation}
    \pi^{new}_k=M_k
\end{equation}

\section{EM Algorithm for Mixtures of Binomial Model with Prior}\label{ap:em2}

\section{OLD}
\subsection{Minimize Expectation}

We are trying to seek $\widehat{\mathcal{M}}\in \mathbb{R}^n$ to minimize:
\begin{equation}
    \E_{r,R}\Big[\big(\widehat{\mathcal{M}}_r-\mathcal{M}(R)\big)^2  \Big]
    =\sum\limits_{r}^{n}\Big[\sum\limits_{R}^{N}{ \big(\widehat{\mathcal{M}}_r-\mathcal{M}(R)\big)^2 P(R|r)} \Big]P(r)
\end{equation}

Minimize each entry:
\begin{equation}
    \widehat{\mathcal{M}}_r = \arg\min_{\widehat{\mathcal{M}}_r}\sum\limits_{R=1}^{N}{\Big(\widehat{\mathcal{M}}_r-\mathcal{M}(R) \Big)^2P(R|r)}
\end{equation}
close form solution is:

\begin{equation}
    \widehat{\mathcal{M}}_r=\sum\limits_{R=1}^{N}{\mathcal{M}(R)}P(R|r)
\end{equation}

Then our estimator for \ref{eq:empirical_metric} is :

\begin{equation}
    \E_{r}[\widehat{\mathcal{M}}_r]=\sum\limits_{r=1}^{n}\sum\limits_{R=1}^{N}{\mathcal{M}(R)}P(r|R)P(R)
\end{equation}

\subsection{MAP for Beta-Binomial Model}\label{ch: MAP}
\subsubsection{Beta-Binomial Model}\label{ch:model_bb}

The model is illustrated in \ref{fig:model_bb}. We assume the parameters:
\begin{equation}
  \theta_u \coloneqq \frac{R_u -1}{N-1} 
\end{equation}
 are sampled from the beta prior:
\begin{equation}
    \theta\sim \mathcal{B}(\alpha, \beta)
\end{equation}
The observations $x_u$ is exactly follow the Beta-Binomial distribution (\ref{ap:bbd}):
\begin{equation}
    x\sim BetaBin(n-1,\alpha,\beta)
\end{equation}

\subsubsection{MAP}
Given the prior parameters $\alpha$ and $\beta$, for each data point $x_u$, we can maximize the posterior to estimate $\theta_u$. From \ref{eq:bb_posterior}, we know posterior of Beta-Binomial distribution is exactly beta distribution, we could directly calculate the mode in our sampling problem scenario:
\begin{equation}\label{eq:map}
    \widehat{\theta}_u = \arg\max P(\theta|x_u) = \frac{x_u+\alpha-1}{n + \alpha+\beta-3}
\end{equation}
\begin{equation}\label{eq:tuRu}
    \widehat{R}_u = (N-1)\widehat{\theta}_u+1
\end{equation}

Then \ref{eq:empirical_metric} can be estimated by:
\begin{equation}\label{eq:MRu}
    \frac{1}{M}\sum\limits_{u=1}^{M}{\mathcal{M}(\widehat{R}_u)}
\end{equation}

This method is denoted as \textbf{MAP}. Note, this method requires the knowledge of beta prior - parameters $\alpha$ and $\beta$.

\subsection{Empirical Bayes for Beta-Binomial Model}

% \begin{figure}[t]
%     \centering
%     \includegraphics[scale = 1]{figure/pre/bb.png}
%     \caption{Graphical representation of Beta-Binomial model, where $u = 1, \dots, M$ denotes different data points.}
%     \label{fig:model_bb}
% \end{figure}
We are still considering the  Beta-Binomial model from \ref{ch:model_bb} in this section.

\subsubsection{Empirical Bayes}

Since $x\sim BetaBin(n-1,\alpha,\beta)$, we could directly get the likelihood function:
\begin{equation}\label{eq:bb_mle}
    \mathcal{L}=\prod_{u=1}^{M}{\binom{n-1}{x_u}\frac{\mathcal{B}(x_u+\alpha,n-1+\beta-x_u)}{\mathcal{B}(\alpha,\beta)}}
\end{equation}

where $\mathcal{B}$ is the beta function:
\begin{equation}\label{eq:beta_fn}
    \mathcal{B}(\alpha, \beta) = \int_0^1{x^{\alpha -1}(1-x)^{\beta-1}dx}, \quad \alpha >0, \beta >0
\end{equation}
Then we can proceed with maximum likelihood estimation of $\alpha$ and $\beta$ based on \ref{eq:bb_mle}.

\begin{equation}\label{eq:ab_mle}
    \widehat{\alpha},\widehat{\beta} =\arg\max_{\alpha,\beta} \mathcal{L}
\end{equation}
Although the $\alpha$ and $\beta$ are not expressible in closed form, we can calculate them numerically or following the method of moment (see \ref{ap:moment}).

\subsubsection{Rank Estimation}\label{ch:rank_bayes}
 Once the estimate value of parameter $\alpha,\beta$ are obtained, the single-prior Bayes estimator ~\ref{point estimation book} of $\theta_u$ under squared error loss is:
\begin{equation}
    \widehat{\theta}_u = \E{[\theta_u|x_u,\widehat{\alpha},\widehat{\beta}]}=\frac{\widehat{\alpha}+x_u}{\widehat{\alpha}+\widehat{\beta}+n-1}
\end{equation}
Then follow the same procedure of \ref{eq:tuRu,eq:MRu} to estimate the global metric. This method we denote as \textbf{BB-\Romannum{1}}.

\subsubsection{Distribution Estimation}\label{ch:distribution_bayes}
Once $\widehat{\alpha}$ and $\widehat{\beta}$ are obtained from \ref{eq:ab_mle}, we have the full knowledge of the distribution of $P(\theta)$.
After a trivial discrete processing, we are able to obtain the probability mass function estimation of $P(R)$:
\begin{equation}
    \widehat{P}(R) = \widehat{P}(\theta_R)  = discrete(P(\theta))
\end{equation}
where 
\begin{equation}
    \theta_R \coloneqq \frac{R-1}{N-1}
\end{equation}

Then we could estimate \ref{eq:empirical_metric}:
\begin{equation}\label{eq: es_pr}
    \sum\limits_{R=1}^{N}{\mathcal{M}(R)\widehat{P}(R)}
\end{equation}

This method we denote as \textbf{BB-\Romannum{2}}.
